# Supplementary material for: Better than Your Teacher: LLM Agents that learn from Privileged AI Feedback
Source: arXiv:2410.05434 source file (2024-10-07)
Supplement: Supplementary file 6 [file trajectories.tex]

\section{Trajectories}
\label{sec:appendix:results}
